# Supplementary material for: Accelerating Distributed MoE Training and Inference with Lina
Source: arXiv:2210.17223 source file (2024-04-28)
Supplement: Supplementary file 1 [file appendix.tex]

\clearpage
\appendix
